# Supplementary material for: CGGT: Curve-Grounded Geometry Transformer for 3D Parametric Curve Reconstruction
Source: arXiv:2609.14521 source file (2026-09-13)
Supplement: Supplementary file 1 [file supp.tex]

\maketitlesupplementary

This supplementary material provides details that complement the experimental section of the main paper. 
We first describe the construction of Wireframe-100K, including the rendering pipeline, camera sampling strategy, and cross-view instance-level curve mask generation. 
We then provide the evaluation protocol, metrics, baseline configurations, and implementation details. 
We further include real-world comparisons and robustness boundary analysis to evaluate the generalization ability and stability of our method under challenging conditions.

\section{Additional Experimental Details}

\subsection{Dataset Construction}

\paragraph{Wireframe-100K}
We construct \textbf{Wireframe-100K}, a large-scale multi-view dataset for data-driven 3D parametric curve reconstruction, based on the ABC dataset~\cite{koch2019abc}. 
The dataset contains 100,000 CAD models with diverse shapes, topologies, and curve structures. 
For each model, we extract its parametric wireframe representation, including line segments, ellipses, and Bézier curves. 
Each curve primitive is assigned a persistent instance ID, which is shared across all rendered views and later used to generate cross-view consistent 2D curve masks.

For each CAD model, we render 50 calibrated RGB-D images at a resolution of $512 \times 512$. 
Each sample contains RGB images, mask images, depth maps, camera intrinsics and extrinsics, 3D parametric curve annotations, and instance-level 2D curve masks. 
The persistent curve IDs allow the same 3D curve to be associated across multiple views, enabling supervised learning of multi-view consistent curve grounding.

\paragraph{Rendering Setup.}
We use BlenderProc~\cite{Denninger2023} to generate realistic multi-view renderings. 
To increase visual diversity and improve generalization, we randomize camera viewpoints, HDR environment lighting, object materials, surface roughness, and texture appearance. 
Objects are placed on a ground plane, whose texture is sampled from CC-Texture~\cite{cc0textures}. 
Object materials and textures are sampled from Poly-Haven~\cite{polyhavenPolyHaven}. 
This rendering strategy produces realistic image observations with varying illumination, material properties, and background appearance, making the training data closer to casual real-world captures.
To generate these views, we randomly sample camera poses looking at the object center, with camera distances ranging from 1.5 to 3.5 meters and elevation angles between 25 and 65 degrees. We will include these specific rendering metrics in the text and open-source our dataset generation code for full reproducibility.

\paragraph{Cross-View Curve Mask Generation.}
To generate 2D supervision, we project each annotated 3D curve into every rendered view using the calibrated camera parameters. 
Visibility is determined by depth-based testing: a projected curve point is considered visible only if its projected depth is consistent with the rendered depth map. 
Visible curve fragments are then rasterized into 2D segmentation masks. 
Each visible pixel is assigned the persistent ID of its corresponding 3D curve primitive. 
As a result, the same curve instance receives consistent labels across different views, while occluded or invisible fragments are excluded from supervision.

This procedure provides accurate instance-level curve masks without relying on 2D edge detectors. 
It also allows the model to learn the distinction between true object-level geometric curves and view-dependent pseudo-edges, such as texture boundaries and silhouette edges.

\subsection{Evaluation Benchmark}

\paragraph{ABC-NEF Evaluation Set.}
For quantitative comparison with prior work, we evaluate our method on the full ABC-NEF benchmark~\cite{Ye_2023_CVPR}. 
The benchmark contains 115 CAD objects with diverse geometries and topologies. 
To ensure a fair comparison, we use the same object set as ABC-NEF for evaluation. 
We re-render these objects under realistic scene settings using the same rendering pipeline as Wireframe-100K. The re-rendered images include randomized camera poses, lighting, object materials, and ground textures, making the evaluation closer to practical casual-capture scenarios.

All methods are evaluated on the same set of objects. 
For methods that require edge maps or masks as input, we provide the corresponding preprocessed edge images following their original settings. 
In contrast, our method directly takes the original RGB images as input and does not require object-mask extraction or edge-map preprocessing.

\subsection{Evaluation Metrics}

We evaluate all methods from three perspectives: reconstruction accuracy, geometric compactness~\cite{Gao_2025_ICCV}, and computational efficiency. Since the baseline methods rely on external 2D edge maps, we use DexiNed~\cite{poma2020dense} as the edge detector, which we found to perform best empirically. 

\paragraph{Reconstruction Accuracy.}
Following established protocols~\cite{Li2024CVPR,Ye_2023_CVPR}, we report Accuracy (Acc.) and Completeness (Comp.) in millimeters. 
Accuracy measures the average distance from reconstructed curve samples to the ground-truth curve samples, while Completeness measures the average distance from ground-truth samples to the reconstructed curves. 
We also report Recall ($\mathrm{R}_{\tau}$), Precision ($\mathrm{P}_{\tau}$), and F-score ($\mathrm{F}_{\tau}$) under distance threshold $\tau$, where distances are computed between sampled points on the reconstructed and ground-truth curves.

\paragraph{Coordinate Alignment.}
Since our method takes unposed images as input, the predicted geometry is defined up to a global similarity transformation. 
Following VGGT~\cite{wang2025vggt}, we align the predicted point cloud to the ground truth using the Umeyama algorithm~\cite{umeyama1991least}, and apply the resulting similarity transformation to the reconstructed 3D curves before evaluation. 
In contrast, the baseline methods are evaluated with ground-truth camera poses following their original settings, and therefore do not require this alignment step.  

\paragraph{Geometric Compactness.}
In addition to reconstruction fidelity, we evaluate geometric compactness following CurveGaussian~\cite{Gao_2025_ICCV}. 
This metric reflects whether the reconstructed wireframe represents the object using a concise set of curve primitives rather than fragmented or redundant curve segments. 
A compact reconstruction is preferred because it better matches editable CAD-style representations.

\paragraph{Computational Efficiency.}
We report the total reconstruction time for each method, including preprocessing, per-scene optimization, and curve fitting when applicable. 
For our method, the reported time includes the feed-forward inference of CGGT and the subsequent fast parametric curve optimization stage.

\subsection{Baseline Methods}

We compare our method with five state-of-the-art curve reconstruction baselines: EMAP~\cite{Li2024CVPR}, SGCR~\cite{yang2025sgcr}, EdgeGaussians~\cite{chelani2024edgegaussians}, CurveGaussian~\cite{Gao_2025_ICCV}, and SketchSplat~\cite{Ying_2025_ICCV}. 
EMAP is a NeRF-based method that reconstructs an implicit edge-aware field and then extracts parametric curves. 
SGCR and EdgeGaussians use 3D Gaussian Splatting to accelerate the reconstruction of geometric boundaries and thin structures. 
CurveGaussian and SketchSplat adopt more direct differentiable rendering formulations to optimize curve-aware primitives from image observations.

For all baselines, we follow the official implementations and recommended hyperparameters whenever available. 
Methods that require precomputed edge maps or masks are provided with the corresponding preprocessed inputs. 
Our method does not use such preprocessing and directly operates on RGB images.

\subsection{Implementation Details}

CGGT is trained on 4 NVIDIA A100 GPUs using AdamW. 
We freeze the pretrained VGGT~\cite{wang2025vggt} backbone, camera head, and depth head, as well as the DINOv2 encoder~\cite{oquab2023dinov2}. 
All remaining modules, including the cross-attention fusion module, pixel decoder, and curve-aware mask transformer decoder, are optimized with a learning rate of $1\times10^{-5}$. 
For each sample, we randomly select one object and sample 2 to 12 views, with a total batch size of 48 images. 
We use 64 curve queries and skip objects with more than 64 curve instances during training. 
Following VGGT, we apply image augmentations including random scaling, cropping, and blur.

For the parametric curve optimization stage, we first back-project the grounded 2D curve pixels into 3D using the predicted depth maps and camera poses. 
RANSAC-based fitting is used to initialize line, ellipse, and Bézier curve candidates. 
We then jointly optimize the parameters of all curves using Adam with a learning rate of $1\times10^{-3}$. 
The optimization runs for 300 iterations and typically converges within approximately 10 seconds on a single GPU.


\subsection{Comparison on Real-World Data}

Real-world datasets pose significant challenges due to uncontrolled lighting, casually captured viewpoints, sensor noise, and cluttered backgrounds. 
To quantitatively evaluate our method in real scenarios, we follow CurveGaussian~\cite{Gao_2025_ICCV} and conduct experiments on six real-world examples from the MV2Cyl dataset~\cite{hong2024mv2cyl}. 
Our method uses 10 input images for each object, while the baseline methods are evaluated with dense-view inputs following their original settings. 
We compare against state-of-the-art methods, including CurveGaussian~\cite{Gao_2025_ICCV} and EdgeGaussians~\cite{chelani2024edgegaussians}.

Following MV2Cyl~\cite{hong2024mv2cyl}, we use ICP to align the reconstructed edge point cloud with the ground-truth CAD model before evaluation. 
As shown in Tab.~\ref{tab:real_demo} and Fig.~\ref{fig:real_demo}, our method achieves higher reconstruction accuracy and more compact 3D edge representations. 
Notably, prior methods mainly rely on geometric fitting without instance-level curve priors, often producing fragmented or redundant curve segments. 
In contrast, our method benefits from instance-level curve grounding, resulting in significantly fewer curve primitives while preserving the underlying object structure.

\begin{table}
\centering
\scalebox{0.80}{
\begin{tabular}{c|cc|ccc|c}
\hline
   Method & Acc. $\downarrow$      & Comp. $\downarrow$ & $\text{R}_{10} \uparrow$  &  $\text{P}_{10} \uparrow$  &  $\text{F}_{10} \uparrow$  &$ N_{\text{curve}}$ $\downarrow$  \\
\hline

EdgeGaussians  &  13.8 &{7.7}& 74.4 & 46.1& 56.7 & 1952.5 \\
CurveGaussian  & {8.5}& 7.8& {74.6}&{ 71.6}& {73.1}& {70.5} \\ 

Ours & {6.3}& 5.9& {81.8}&{ 78.5}& {79.4}& {21.3} \\ 
\hline
\end{tabular}
}
\caption{\textbf{Quantitative comparisons on  MV2Cyl's real objects.} 
}

\label{tab:real_demo}

\end{table}


\begin{figure}[t]
  \centering
  \includegraphics[width=1.0\linewidth]{figs/real_com.pdf}
  \caption{\textbf{Qualitative comparison on real-world data.}
  Our method effectively grounds 2D curve instances and reconstructs the final 3D wireframes.
  Note that object masks are used only to filter background detections.}
  \label{fig:real_demo}
\end{figure}


\subsection{Robustness Boundary Analysis}

Our framework relies on the first-stage CGGT predictions, including camera poses, depth maps, curve masks, and cross-view curve correspondences. 
When the geometry estimated by the 3D foundation model is severely inaccurate, the subsequent 3D lifting and parametric optimization stages can also be affected. 
To better understand the robustness boundary of our method, we conduct controlled perturbation experiments on the Phase I outputs and input images. 
Starting from the original performance of the full model, i.e., $\mathrm{R}_{10}=73.6$, $\mathrm{P}_{10}=76.3$, and $\mathrm{F}_{10}=74.5$, we evaluate four types of perturbations at three levels: 5\%, 10\%, and 20\%.

Specifically, we consider: 
(1) adding geometric noise to the predicted poses and depth maps; 
(2) randomly deleting curve-mask pixels to simulate missed curve detections; 
(3) randomly shuffling curve correspondences across views to simulate instance matching errors; and 
(4) adding Gaussian noise to the input images to evaluate robustness to image degradation. 
The results are shown in Fig.~\ref{fig:robustness_boundary}.

\paragraph{Geometry noise.}
Geometry noise has a relatively strong impact on the final reconstruction quality. 
This is expected, since inaccurate poses or depth maps directly affect the 3D lifting process and the subsequent parametric fitting. 
However, this is not a fundamental limitation of the proposed curve grounding formulation. 
Our main contribution is to provide multi-view consistent curve masks and curve correspondences in the image space. 
Since CGGT builds upon a 3D foundation model, it can naturally benefit from future advances in feed-forward 3D reconstruction, which would further improve the downstream 3D curve reconstruction quality.

\paragraph{Curve-mask deletion.}
Randomly deleting curve-mask pixels causes only moderate degradation, especially at low perturbation levels. 
This robustness comes from the multi-view nature of our framework: even if a curve is partially missed in some views, observations from other views can still provide sufficient evidence for 3D lifting and fitting. 
This result suggests that the parametric optimization stage can tolerate moderate mask incompleteness.

\paragraph{Curve correspondence errors.}
Shuffling a small portion of curve correspondences has limited impact at 5\% and 10\%, indicating that the optimization can absorb moderate correspondence noise through multi-view consistency. 
However, the degradation becomes significant at 20\%. 
This is because incorrect cross-view curve correspondences introduce direct constraint noise into the second-stage optimization, causing unrelated 2D observations to be fitted as the same 3D curve. 
This result highlights the importance of reliable instance-level curve association.

\paragraph{Image Gaussian noise.}
Adding Gaussian noise to the input images has the mildest effect among the four perturbations. 
We attribute this robustness to the large-scale training of CGGT and the image augmentations used during training, including random scaling, cropping, and blur. 
These augmentations help the model learn stable curve-level priors beyond local pixel noise.

Overall, the analysis shows that our framework is robust to moderate mask incompleteness, image degradation, and limited correspondence noise, while being more sensitive to severe geometric errors. 
This behavior is consistent with our two-stage design: the first stage focuses on image-space curve grounding, whereas the second stage relies on accurate geometry for 3D lifting and parametric refinement.

\begin{figure}[t]
  \centering
  \includegraphics[width=1.0\linewidth]{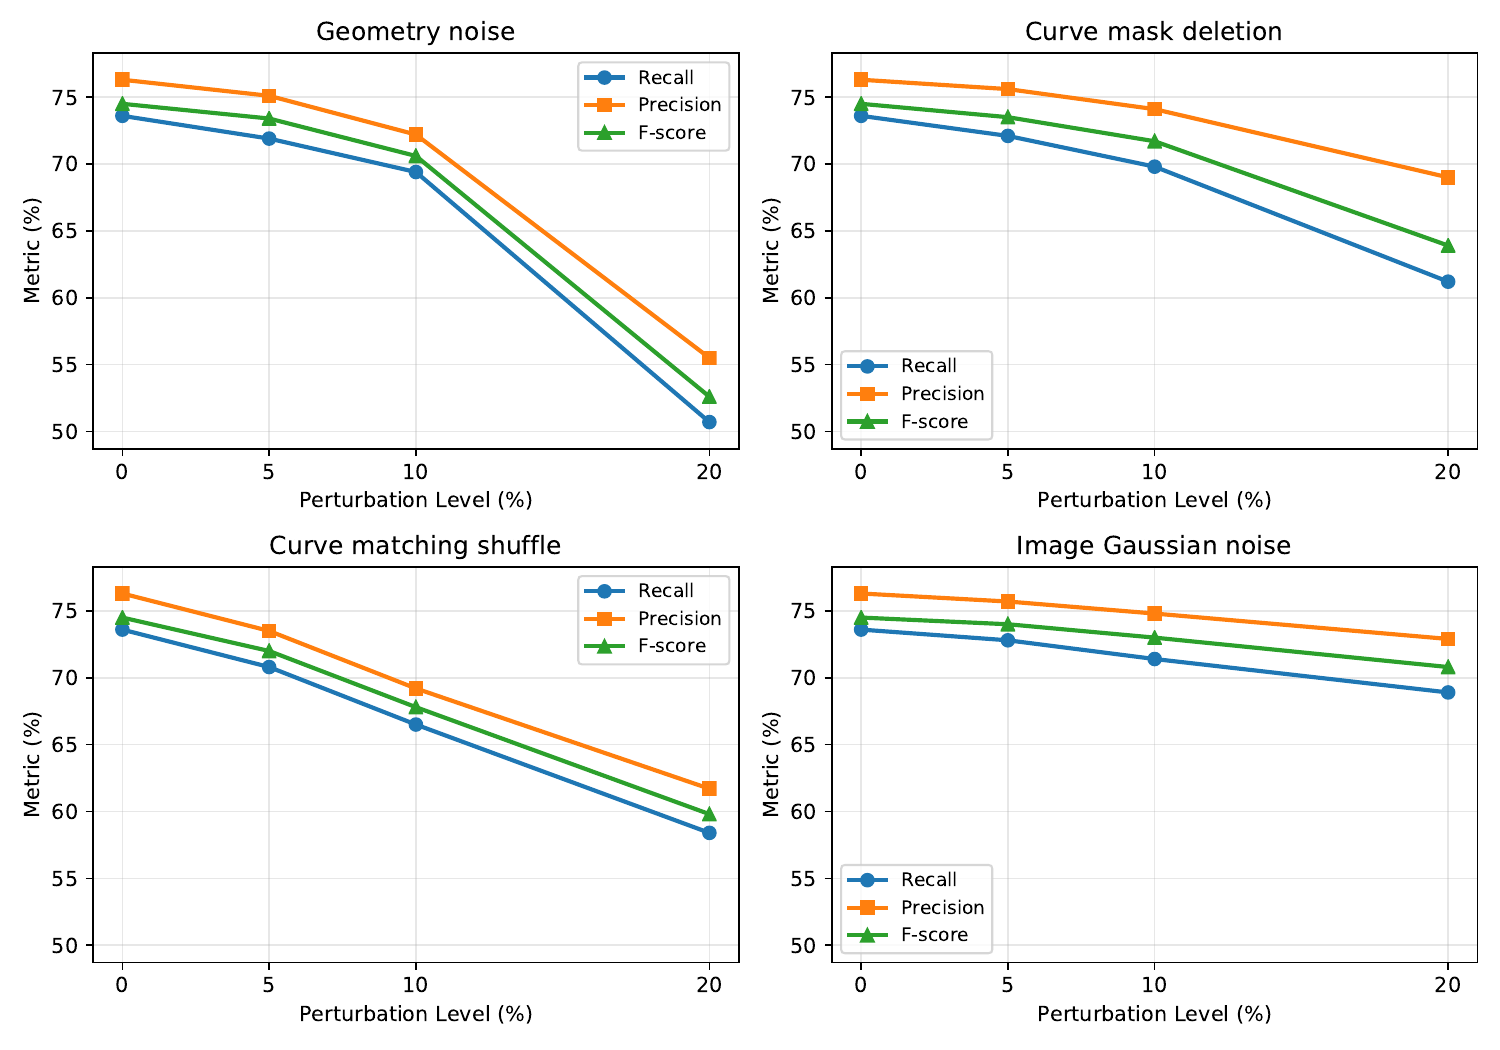}
  \caption{\textbf{Robustness boundary analysis.}
  We perturb Phase I predictions and input images at 5\%, 10\%, and 20\% levels.
  Our method is relatively robust to image noise, curve mask deletion, and limited correspondence errors, but is more sensitive to geometry noise because pose and depth errors directly affect 3D lifting and parametric fitting.}
  \label{fig:robustness_boundary}
\end{figure}
